# Supplementary material for: Exploiting Hierarchy for Learning and Transfer in KL-regularized RL
Source: arXiv:1903.07438 source file (2020-01-23)
Supplement: Supplementary file 1 [file neurips_2019_appendix.tex]

\documentclass{article}

% if you need to pass options to natbib, use, e.g.:
     \PassOptionsToPackage{numbers, compress}{natbib}
% before loading neurips_2019

% ready for submission
%\usepackage{neurips_2019}

% to compile a preprint version, e.g., for submission to arXiv, add add the
% [preprint] option:
%     \usepackage[preprint]{neurips_2019}

% to compile a camera-ready version, add the [final] option, e.g.:
    %  \usepackage[final]{neurips_2019}

% to avoid loading the natbib package, add option nonatbib:
\usepackage[nonatbib]{neurips_2019}

\usepackage[utf8]{inputenc} % allow utf-8 input
\usepackage[T1]{fontenc}    % use 8-bit T1 fonts
\usepackage{hyperref}       % hyperlinks
\usepackage{url}            % simple URL typesetting
\usepackage{booktabs}       % professional-quality tables
\usepackage{amsfonts}       % blackboard math symbols
\usepackage{nicefrac}       % compact symbols for 1/2, etc.
\usepackage{microtype}      % microtypography

% Custom packages
%\usepackage{floatrow}
\usepackage{amsmath,amssymb}
\usepackage{mathtools}
\usepackage{color}
\usepackage{dsfont}
\usepackage{wrapfig}
\usepackage{graphicx}
\usepackage{subfigure}
\usepackage[rightcaption]{sidecap}    
\sidecaptionvpos{figure}{t}

\usepackage{caption}

\usepackage{algorithm}
\usepackage{algorithmic}

\newcommand{\appendixenvironments} E
\newcommand{\appendixexperimentalsettings} F

\newcommand{\appendixhyperparameters} G

\title{Exploiting Hierarchy for Learning and\\ Transfer in KL-regularized RL \\ {\Large Supplementary Material}}

% The \author macro works with any number of authors. There are two commands
% used to separate the names and addresses of multiple authors: \And and \AND.
%
% Using \And between authors leaves it to LaTeX to determine where to break the
% lines. Using \AND forces a line break at that point. So, if LaTeX puts 3 of 4
% authors names on the first line, and the last on the second line, try using
% \AND instead of \And before the third author name.

\author{%
  David S.~Hippocampus\thanks{Use footnote for providing further information
    about author (webpage, alternative address)---\emph{not} for acknowledging
    funding agencies.} \\
  Department of Computer Science\\
  Cranberry-Lemon University\\
  Pittsburgh, PA 15213 \\
  \texttt{hippo@cs.cranberry-lemon.edu} \\
  % examples of more authors
  % \And
  % Coauthor \\
  % Affiliation \\
  % Address \\
  % \texttt{email} \\
  % \AND
  % Coauthor \\
  % Affiliation \\
  % Address \\
  % \texttt{email} \\
  % \And
  % Coauthor \\
  % Affiliation \\
  % Address \\
  % \texttt{email} \\
  % \And
  % Coauthor \\
  % Affiliation \\
  % Address \\
  % \texttt{email} \\
}

\begin{document}

\maketitle

\appendix

\input{arxiv_sections/appendix/alternatives.tex}
\input{arxiv_sections/appendix/algorithm.tex}
\input{arxiv_sections/appendix/derivations.tex}
\input{arxiv_sections/appendix/additional_results.tex}
\input{arxiv_sections/appendix/experimental_setting.tex}

\medskip

\small
\bibliography{neurips2019}
\bibliographystyle{ieeetr}

\end{document}
